# Supplementary material for: A topological transistor of waves via the Euler characteristic
Source: arXiv:1702.01884 source file (2017-02-07)
Supplement: Supplementary file 1 [file DopplerTrt_Supplement.pdf]

# A topological transistor of waves via the Euler characteristic
# Supplementary Material

Sophia R. Sklan and Baowen Li
*Department of Mechanical Engineering, University of Colorado Boulder, Colorado 80309 USA*

## BIFURCATIONS

The propagating modes in the ring are defined by the relation

$$\omega - qR\Omega = \omega_q \equiv 2\sqrt{\frac{k}{m}}\left|\sin\frac{qa}{2}\right| \tag{1}$$

($\Omega$ is rotational velocity) which we can evaluate graphically by locating the intersection of the two curves. The number of intersections changes under two circumstances. First, when $qa = 2\pi * p$ for integer $p$, the Doppler shifted frequency intersects with the Gamma point and so the transistor undergoes a transcritical bifurcation This occurs for a driving frequency $\omega$=$Np\Omega$. More generally, this class of bifurcation occurs whenever the Doppler shifted frequency intersects with a band crossing. Second, when the Doppler shifted frequency intersects tangentially with the dispersion, the system undergoes a saddle node bifurcation. This can only be determined numerically because the dispersion is a transcendental equation. Fourier transforming the numerical solution in the ring, gives clear evidence of this bifurcation, as shown in Figure S1. We can also numerically calculate the number of solutions for a given combination of $\omega$ and $\Omega$, allowing us to construct a phase diagram of the number of states versus rotational velocity and driving frequency. This is shown (only including positive frequency branches) in Figure S2

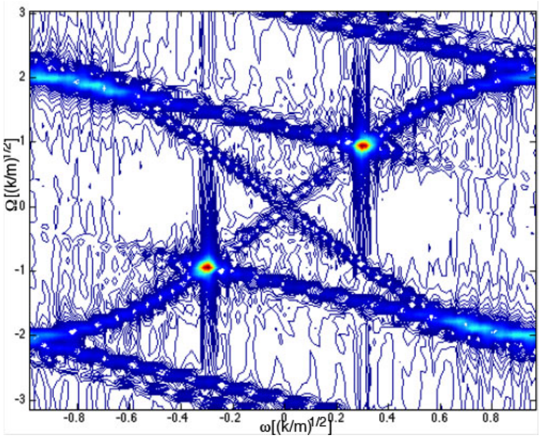


FIG. S1: Spatio-temporal Fourier transform of the numerical solution calculated inside of the ring, displayed as a contour plot. The contour plot retains very small terms, which are several orders of magnitude lower than the peak amplitude but reveal the Doppler shifted and dispersion relation contours described by equation 1. The number of lattice sites, driving frequency, and rotational velocity used here are such that system is undergoing a saddle node bifurcation (extended peak near the band edge).

## RECTIFICATION

Because there are two output branches (i.e. two drains), we are interested in not only how large the transmission is, but also whether there is preferential transmission along one path or the other. Alú et al. [1] used a similar setup, albeit without dispersion, to construct an acoustic circulator (a series of diodes joined in a ring), so it is natural to anticipate a similar phenomenon here. However, because the propagating modes are now the solutions to a transcendental equation, this requires numerical analysis. We numerically integrate the equations of motion, using an input signal of a constant harmonic driving force applied to innermost element of the source waveguide (the damping, necessary to simulate an infinite domain, precludes the application of force at the far end). We define the rectification parameter

$$\mathcal{R} = \frac{\langle U^{(1)}\rangle - \langle U^{(2)}\rangle}{\langle U^{(1)}\rangle + \langle U^{(2)}\rangle} \tag{2}$$

where the brackets refer to the rms average over time of the first lattice site of the respective branch (see lower box of Fig S3). Figure S3 shows the resulting rectification curves as a function of driving frequency $\omega$ for various rotational velocities $\Omega$. As expected, there is very little recitification for the stationary case (dark blue curve) or for constant $\omega = 0$ driving, however there is very clear rectification in the other cases. In some cases this exceeds a rectification factor of 0.9, showing very clear preferential transmission along one of the drains. The presence of the local minima and the saturation can be qualitatively understood in terms of the bifurcations, as explored in the Supplement. In addition, in the inset of Figure S3 we plot the rectification as a function of rotational velocity for a single driving frequency (the curve does not greatly change with the choice of driving frequency). The change of sign of the rectification parameter is to be expected, given that the driving force will set up a standing wave pattern within the ring, which will be shifted by imposed rotation.

## RECTIFICATION & BIFURCATIONS

Figure S4 overlays a contour plot of the rectification over the phase diagram of Figure S2. This reveals that the local minima occurs near a saddle node bifurcation where the system possesses only a small number of propagating modes (two

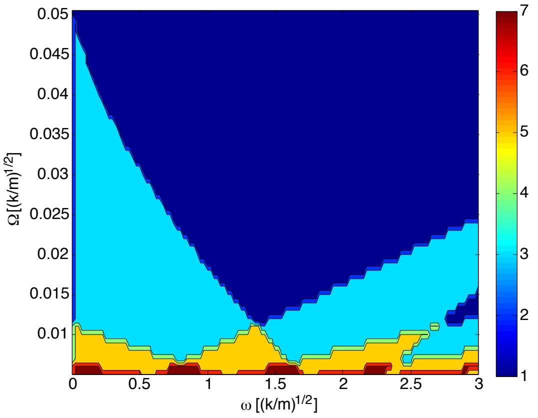


FIG. S2: Phase diagram of the number of propagating positive frequency modes in the ring as a function of driving frequency $\omega$ and rotational velocity $\Omega$.

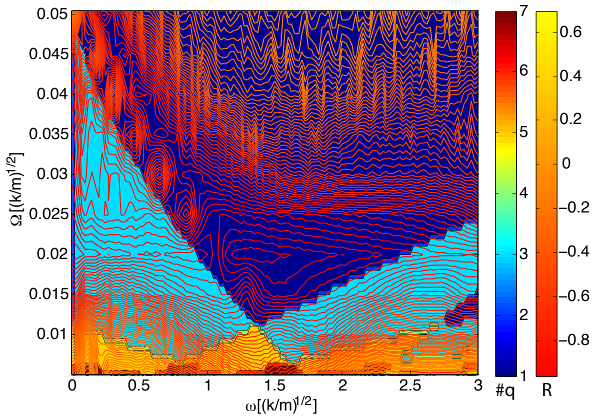


FIG. S4: Overlay of the rectification contour plot on the phase diagram.

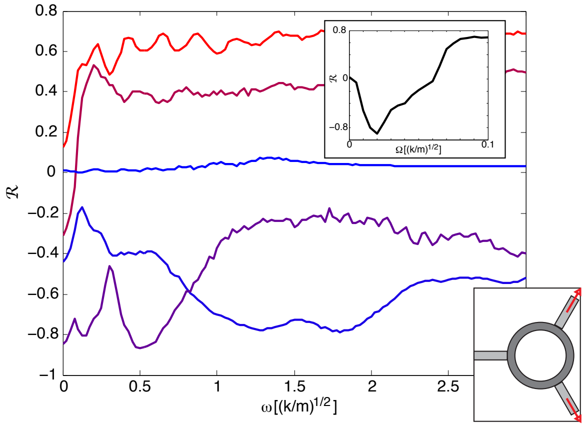


FIG. S3: Rectification of the transmitted signal as a function of driving frequency $\omega$. Color denotes rotational velocity $\Omega$, which varies smoothly between 0 and 0.1 $\sqrt{k/m}$. (Inset) Rectification versus rotational velocity for a single driving frequency . (lower box) Schematic of rectification geometry.

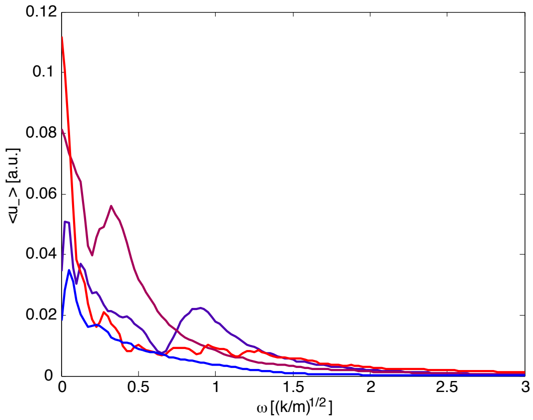


FIG. S5: Transmitted amplitude as a function of driving frequency $\omega$ for a given rotational velocity ($\Omega$, denoted by color and varying smoothly between 0 and $0.1\sqrt{k/m}$).

to four). Near the bifurcation but not at it, there therefore exists a pair of closely spaced solutions that will interfere with each other, promoting rectification. Saturation is found when only one solution propagates, as there are no other modes to interfere with. The variation in rectification is then much slower as a function of driving frequency while being fairly insensitive to rotational velocity.

## TRANSMISSION

The absolute transmission is shown in Figure S5. Qualitatively, we can understand it by considering a damped driven SHO

$$m\ddot{u} + \gamma\dot{u} + ku = Fe^{i\omega t}. \tag{3}$$

If $\omega = \sqrt{k/m}$, then

$$u(t) = \frac{F}{i\gamma\omega}e^{i\omega t}, \tag{4}$$

which falls off rapidly with increasing $\omega$.

[1] R. Fleury, D. L. Sounas, C. F. Sieck, M. R. Haberman, A. Alù, *Science* **343**, 516 (2014).
